# Supplementary material for: Thermal runaway of silicon-based laser sails
Source: arXiv:2110.06185 ancillary file (2021-10-12)
Supplement: Supplementary file 1 [file Si_Laser_Sail_Heating_Supplement.pdf]

# Supporting Information
## Thermal runaway of silicon-based solar sails


Gregory R. Holdman* and Gabriel R. Jaffe,[1,*] Min Seok Jang,[2]
Demeng Feng and Mikhail A. Kats,[3] and Victor Watson Brar[†,1]

[1] *Department of Physics, University of Wisconsin-Madison, Madison WI 53706 USA*
[2] *School of Electrical Engineering, Korea Advanced Institute of Science and Technology, Daejeon 34141, Korea*
[3] *Department of Electrical and Computer Engineering, University of Wisconsin-Madison, Madison WI 53706 USA*

*The authors contribute equally to this paper.
†Email: vbrar@wisc.edu


## I. MODELING OF THE SI ABSORPTION COEFFICIENT

The composite absorption model for Si presented in Fig. 2 of the main text includes two different models of the free carrier absorption coefficient, $\alpha_{FC}$. The model from Ref. [1] is used for wavelengths of 1.45-4 $\mu$m, the model from Ref. [2] is used from 5–100 $\mu$m. Because both models appear to be equally good and we expect the wavelength dependence of the free-carrier absorption to be a smooth function, we perform a linear interpolation between the two models from 4–5 $\mu$m in order to avoid an unphysical discontinuity. These models are shown in Fig. S1 without the interpolation as dashed black lines. The thin solid black line denotes the absorption below 1.45 $\mu$m from Ref. [3] and the thick black line is the multi-phonon absorption data from Ref. [4, 5]. To our knowledge, the lowest demonstrated absorption of Si at 1.55$\mu$m is $4.28\times10^{-6}$ cm$^{-1}$ and is denoted in Fig. S1 as a solid black circle and labeled as 'Hero Si'.[6] The absorption of Si from 7–100 $\mu$m, which at room temperature is dominated by multi-phonon absorption, has been measured; however, the tail from these absorption bands at wavelengths shorter than 7 $\mu$m has not.[4, 5]

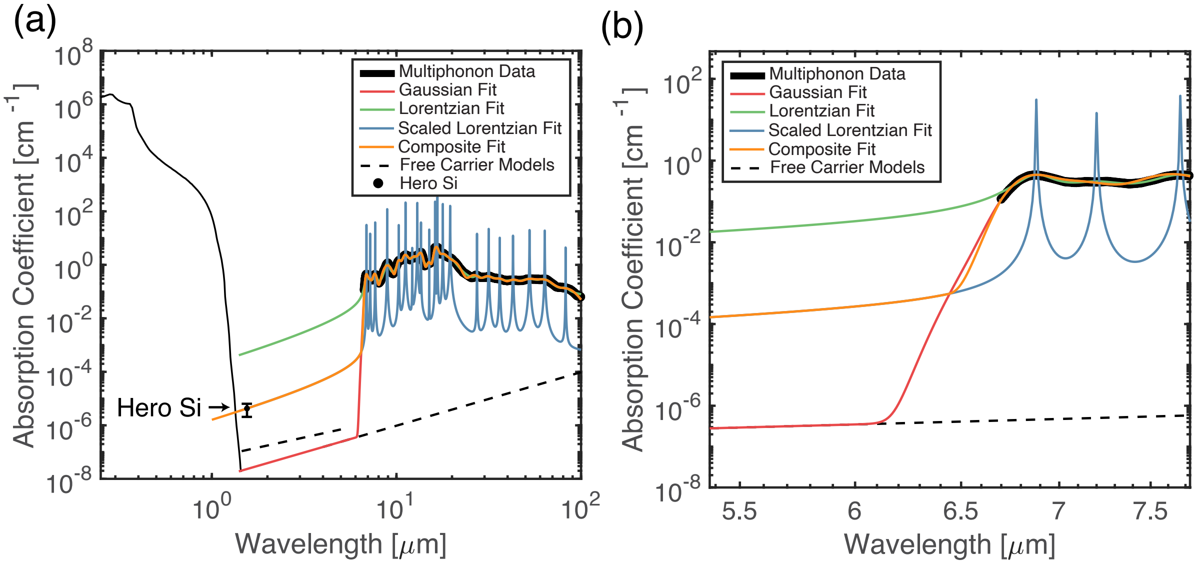


*

Figure S1. (a) The absorption of Si as a function of wavelength. Literature data and models of the absorption are shown as black lines and circles.[1–6]. Fits to the multi-phonon data assuming either Lorentzian or Gaussian peaks are shown in green and red, respectively. Note, the orange, green and red curves overlap at wavelengths $>7\,\mu$m. Scaling the Lorentzian fit peak widths such that the tail passes through the Hero Si data point at $1.55\,\mu$m produces the blue curve. The composite model used in the calculations in the main text consists of the scaled Lorentzian fit at short wavelengths and the Guassian fit at long wavelengths and is shown in orange. The orange and blue curves overlap below $6.43\,\mu$m. (b) The absorption data and fits pictured in (a) over a narrower wavelength range. The composite fit (orange) linearly interpolates between the scaled Lorentzian fit (blue) and Gaussian fit (red) from 6.43–6.70 $\mu$m.

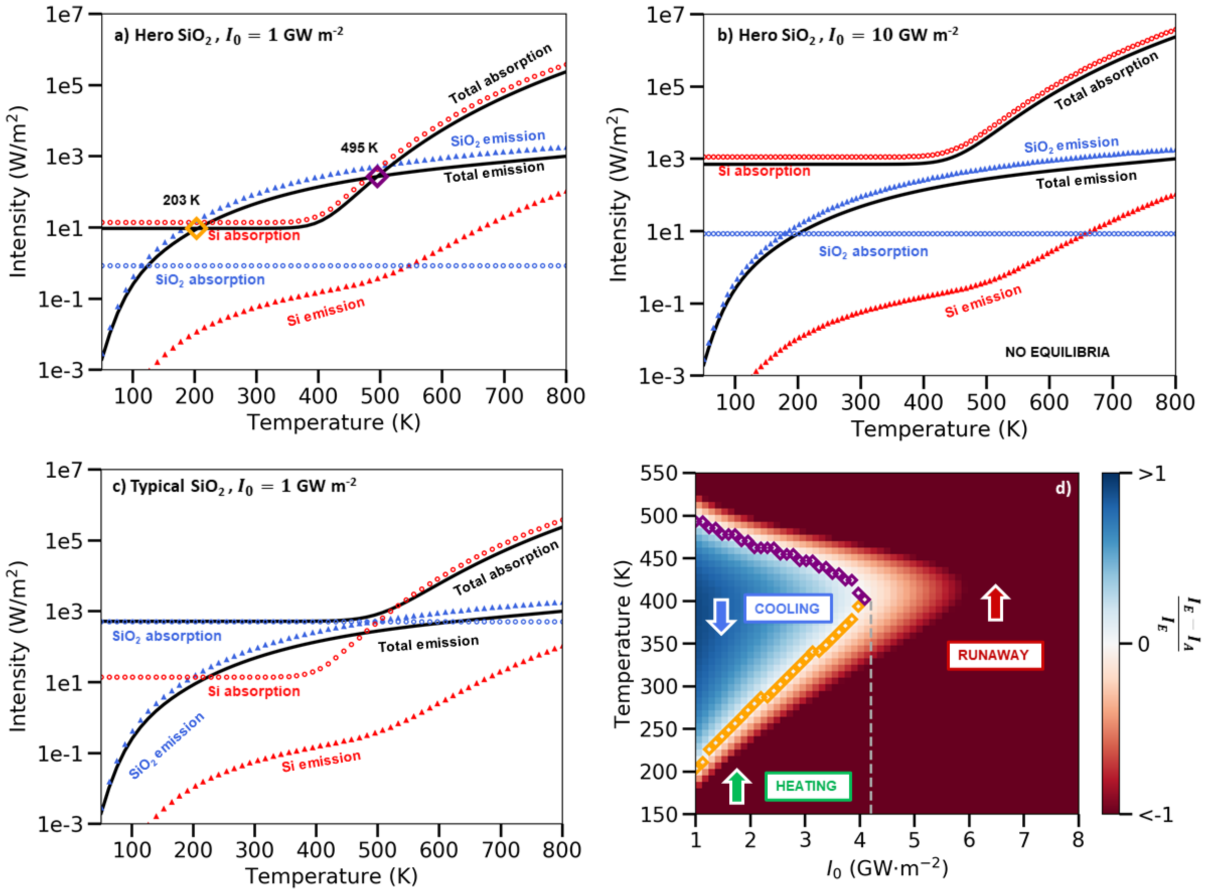


Figure S2. Replication of Fig. 3 in the main text, but for a Si/$SiO_2$ heterostructure with a solid layer of 450 nm Si on 200 nm $SiO_2$. (a-c) Absorbed and thermally emitted intensities versus temperature for the Si/$SiO_2$ heterostructure made from either Hero or Typical $SiO_2$ and illuminated with an incident laser intensity $I_0$. Stable (orange) and unstable (purple) equilibrium temperatures are labeled as diamonds. Note, there is no equilibrium temperature for Typical $SiO_2$ at $I_0 = 1\,\mathrm{GW{\cdot}m^{-2}}$ or Hero $SiO_2$ at $I_0 = 10\,\mathrm{GW{\cdot}m^{-2}}$. Absorbed and emitted intensities for the complete laser sail are shown in black while the contribution of the Si and $SiO_2$ layers are shown in red and blue, respectively. Dotted lines are used to indicate the Si absorption and $SiO_2$ emission because they overlap with the total absorption and emission. (d) Normalized difference in emissive intensity and absorptive intensity as a function of temperature $T$ and incident intensity $I_0$ for a sail made with Hero $SiO_2$. Stable and unstable equilibrium temperatures are indicated as orange and purple diamonds, respectively. The blue and green arrows indicate the zones where the sail will either cool or heat to a stable equilibrium temperature below $I_0 \approx 4.1\,\mathrm{GW{\cdot}m^{-2}}$. Otherwise, thermal runaway occurs.

We fit the multiphonon absorption peaks with Lorentzian lineshapes in order to extrapolate between the short-wavelength edge of the multiphonon data at $7\mu$m and the measured absorption at $1.55\,\mu$m. First, the absorption contribution from free carriers is subtracted from multiphonon resonances. A least-squares fit is performed using Lorentzians centered at each of the allowed two- and three-phonon absorption peaks, and the carbon impurity peak.[5, 7] Additional absorption peaks at 20, 27, 32, 36, 43, 53, 64, and $82\,\mu$m were included in the fit to better match the absorption features seen in the data at long wavelengths. We note that these energies are too small to arise from multi-phonon absorption processes and that the multi-phonon and carbon impurity peaks are the dominant contributors to the absorption tail at $1.55\,\mu$m. The tail of the best fit Lorentzian model (green curve in Fig. S1) predicts absorption

several orders of magnitude above the measured Hero Si absorption. This indicates that the width of the peaks in the multiphonon data is the result of inhomogeneous broadening. The broadened Lorentzian peaks will appear Guassian near the center of each peak. A fit using Gaussian lineshapes instead of Lorentzians (red curve) matches the data well near the peaks but decays too rapidly at short wavelengths to capture the expected long tail behavior of Lorentzians. We therefore scale the widths of the peaks in the best fit Lorentzian model until the tail passes through the Hero Si absorption data point at 1.55 $\mu$m (blue curve). The model for the multi-phonon absorption coefficient, $\alpha_L(\lambda)$, as a function of wavelength, $\lambda$, used in the main text consists of the scaled Lorentzian fit for $\lambda$ <6.43 $\mu$m, the best fit Gaussian model for $\lambda$ >6.70 $\mu$m, and then a linear interpolation between the two fits from 6.43–6.70 $\mu$m. This composite fit is shown in orange in Fig. S1.

## II. COMPARISON OF THE EMISSION AND ABSORPTION OF THE METASURFACE TO A CONTINUOUS SLAB

In the main text, we showed that a particular highly reflective metasurface will experience thermal runaway at all incident intensities $I_0 > 5.4\,\mathrm{GW{\cdot}m^{-2}}$. In this section, we perform the same analysis on a heterostructure of 450 nm of Si on 200 nm of SiO2. The layer thicknesses of this heterostructure are identical to those of the the metasurface we analyzed in the main text; however, the Si layer in the heterostructure is a continuous slab instead of individual blocks. We find that the heterostructure geometry also exhibits the thermal runaway behavior of the metasurface, and has an even lower maximum $I_0$, above which no equilibrium temperature exists.

The emission intensity $I_E$ is calculated in the same way as described in the main text while absorption $I_A$ is now calculated analytically, since the surface is translationally invariant. We plot the results in Fig. S2. We see that for the high-quality Hero $SiO_2$ and $I_0 = 1\,\mathrm{GW{\cdot}m^{-2}}$, the stable temperature has risen to 203 K from the 177 K of the metasurface, while the unstable temperature has lowered to 495 K from 516 K. In Fig. S2d, we see this also has the effect of lowering the incident intensity limit to $I_0 = 4.1\,\mathrm{GW{\cdot}m^{-2}}$. The heterostructure is less thermally robust than the metasurface because the total absorption in the Si has risen slightly from the increased surface coverage.

The acceleration distance of the heterostructure sail design suffers for two reasons. First, as seen in Fig. S2d, the maximum $I_0$ the heterostructure can withstand is lower than that of the metasurface in the main text. Second, it is far from being highly reflective across the Doppler band of interest. Using the reflectivity spectrum and $I_0 = 4.1\,\mathrm{GW{\cdot}m^{-2}}$, we calculate the acceleration distance to be $D$ =532 Gm. This is more than 4 times larger than the 120 Gm acceleration distance of the metasurface in the main text.

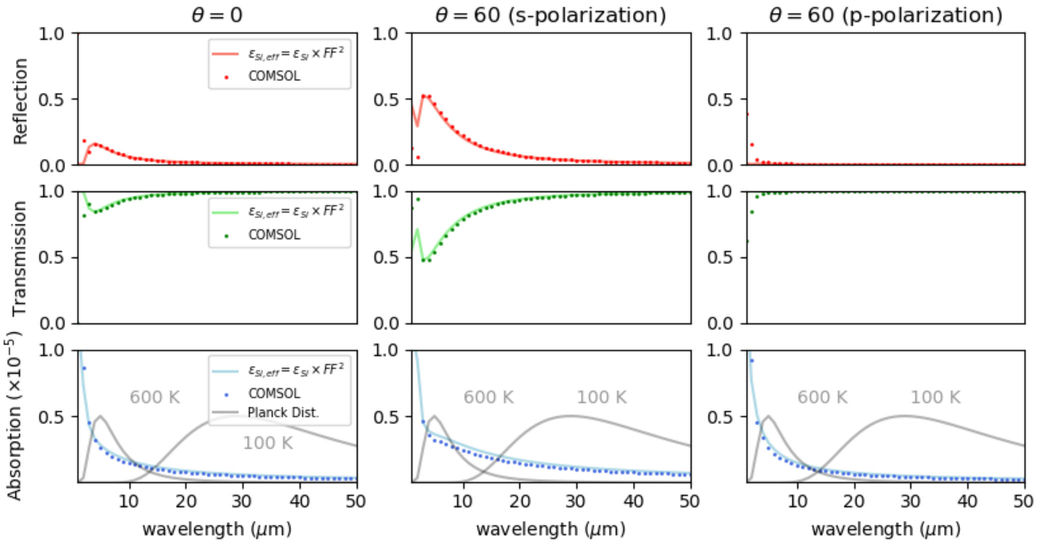


Figure S3. Comparison of the reflection, transmission, and absorption spectra of the metasurface using the analytic approximation (i.e. assuming Si to be a solid slab with an effective index) and full-wave simulations in COMSOL. For wavelengths longer than 2 $\mu$m, the agreement is very good, implying that this approximation is valid for calculations of the metasurface's emissivity.

## III. EFFECTIVE MEDIUM APPROXIMATION IN MID-INFRARED AND BEYOND

The calculation of $I_E(T) = I_E^s(T) + I_E^i(T)$, requires performing an integration over all wavelengths, angles, and polarizations of interest using the formula

$$I_E^i(T) = \int_{\lambda_1}^{\lambda_2} d\lambda \int_0^{2\pi} d\phi \int_0^{\pi} d\theta \quad \epsilon_i(\lambda, \phi, \theta, T) \frac{hc^2}{\lambda^5} \frac{1}{\exp(hc/\lambda k_B T) - 1} \cos\theta \sin\theta, \quad (i = s, p). \tag{1}$$

The emissivity $\epsilon_i(\lambda, \theta, \phi)$ $(i = s, p)$ varies as a function of $\lambda$, $\theta$, $\phi$, and $i$. To perform this calculation by sweeping the parameters in COMSOL would be extremely computationally intensive.

To simplify this calculation, we approximate the emissivity by replacing the blocks of Si with a slab of equal thickness 450 nm and refractive index $n_{eff} = n_S i \times FF$ where $FF = (430^2)/(670^2)$ is the filling factor. The geometry in this approximation is then a stack of two unpatterned slabs which has an analytical solution for the absorptivity $\alpha_i(\lambda, \phi, \theta, T)$ using transfer matrices. Using Kirchoff's law of thermal radiation, we obtain $\epsilon_i(\lambda, \phi, \theta, T) = \alpha_i(\lambda, \phi, \theta, T)$ analytically.

At mid-infrared to long-wave infrared wavelengths ( 2-100 $\mu$m where thermal emission occurs), this approximation is valid. We have checked the validity of this approximation by comparing Python-based transfer matrix code with full-wave COMSOL simulations of the metasurface. We used indices $n_{Si} = 11.7 + i10^{-5}$ and $n_{SiO_2} = 2.1 + i10^{-5}$ for Si and $SiO_2$, respectively. Simulations were performed at incident angles $\theta = 0°$ and $60°$, polarizations $s$ and $p$, and from $\lambda = 1$ to 50 $\mu$m. The reflection, transmission, and absorption were recorded as shown in Fig. S3. It is clear that the approximation aligns closely with the simulated result. Some deviation occurs below 2 $\mu$m in wavelength, but this does not significantly affect the calculation of $I_E(T)$ because the blackbody spectrum is quite weak at those wavelengths.


[1] H. Rogne, P. J. Timans, and H. Ahmed, Infrared Absorption in Silicon at Elevated Temperatures, Applied Physics Letters **69**, 2190 (1996), https://doi.org/10.1063/1.117161.

[2] D. K. Schroder, R. N. Thomas, and J. C. Swartz, Free Carrier Absorption in Silicon, IEEE Journal of Solid-State Circuits **13**, 180 (1978).

[3] M. A. Green, Self-Consistent Optical Parameters of Intrinsic Silicon at 300K Including Temperature Coefficients, Solar Energy Materials and Solar Cells **92**, 1305 (2008).

[4] F. A. Johnson, Lattice absorption bands in silicon, Proceedings of the Physical Society **73**, 265–272 (1959).

[5] E. J. Wollack, G. Cataldo, K. H. Miller, and M. A. Quijada, Infrared properties of high-purity silicon, Optics Letters **45**, 4935 (2020).

[6] J. Degallaix, R. Flaminio, D. Forest, M. Granata, C. Michel, L. Pinard, T. Bertrand, and G. Cagnoli, Bulk optical absorption of high resistivity silicon at 1550 nm, Opt. Lett. **38**, 2047 (2013).

[7] M. Pradhan, R. Garg, and M. Arora, Multiphonon infrared absorption in silicon, Infrared Physics **27**, 25 (1987).
